# Supplementary material for: Active topological strings in renewing nematopolar fluids
Source: arXiv:2601.18307 ancillary file (2026-01-26)
Supplement: Supplementary file 1 [file SM.pdf]

# Supplemental Material for
# "Active topological strings in renewing nematopolar fluids"

Alberto Dinelli, Ludovic Dumoulin, and Karsten Kruse
*Department of Biochemistry, University of Geneva, 1211 Geneva, Switzerland and*
*Department of Theoretical Physics, University of Geneva, 1211 Geneva, Switzerland*
(Dated: January 23, 2026)

**Contents**

SI. Hydrodynamics of an active nematopolar fluid 2

SII. Numerical solution of the dynamic equations 4
A. Integration scheme 4
B. Initial conditions 4
C. Data analysis 5

SIII. Equilibrium behavior of nematopolar systems 5
A. Homogeneous and distortion-free configurations 6
B. Topological constraints and string-length selection. 6

SIV. Mechanical properties of active nematopolar fluids with renewal 7
A. Hydrostatic pressure associated with topological point defects 8
B. Anti-symmetric Ericksen stress 8
C. Bulk compressibility and conditions for mechanical stability 9

SV. Green function for Brinkmann-Darcy flow 10

SVI. Hydrodynamic forces and material fluxes 11

SVII. Linear stability analysis in the presence of activity 11

SVIII. Movies 12

References 13

The Supplemental Material (SM) contains details on the derivation of the theoretical and numerical results presented in the main text. In all the SM, Eq. (X) and Fig. X refer to equations and figures of the main text while Eq. (S.X) and Fig. SX refer to equations and figures that appear in the Supplemental Material.

In Sec. SI, we derive the hydrodynamic equations for an active nematopolar fluid. In Sec. SII, we provide details on the numerical methods, initial conditions for simulations and on the data analysis pipeline. The equilibrium behavior of the fluid is then described in Sec. SIII, together with predictions and measurements of the topological string length in the absence of renewal. In Sec. SIV, we derive the expressions for the pressure and anti-symmetric Ericksen stress presented in the main text. We also discuss the condition for mechanical stability. The Green function for the viscous Darcy-Brinkman flow is computed in Sec. SV and the hydrodynamic forces and material fluxes are analyzed in the presence and the absence of renewal in Sec. SVI. In Sec. SVII, we discuss the linear-stability analysis of polarized profiles in the presence of active stresses. Finally, in Sec. SVIII, we report all captions and parameters for the Supplementary Movies.

## SI. Hydrodynamics of an active nematopolar fluid

In this Section we detail the equations governing the hydrodynamics of an active nematopolar fluid in $2d$. We define the polar field as a vector field with components $p_\alpha = p\hat{p}_\alpha$, where Greek indices take the values $x$ and $y$, $p$ denotes the order parameter, and $\hat{p} := (\cos\nu, \sin\nu)$. The symmetric traceless nematic tensor is defined as

$$\mathsf{Q} = \begin{pmatrix} Q_{xx} & Q_{xy} \\ Q_{xy} & Q_{yy} \end{pmatrix} = \frac{S}{2}\begin{pmatrix} \cos 2\psi & \sin 2\psi \\ \sin 2\psi & -\cos 2\psi \end{pmatrix}, \tag{S.1}$$

where $S \geq 0$ represents the nematic order parameter and $\psi$ the local orientation of the nematic director $\hat{n} = (\cos\psi, \sin\psi)$. To simplify notation, we introduce $Q_1 \equiv Q_{xx} = -Q_{yy}$ and $Q_2 \equiv Q_{xy} = Q_{yx}$. Following [1], we describe the free energy $\mathcal{F}$ of the system by

$$\mathcal{F} = \int \mathrm{d}^2\mathbf{r}[f_\rho + f_p + f_Q + f_{pQ}]\ , \tag{S.2}$$

where the contributions to the free energy density read

$$f_\rho = \frac{a}{4}\rho^4 \tag{S.3}$$

$$f_p = \rho^2\left[-\frac{\alpha_p}{2}\frac{\rho}{\rho_0}p^2 + \frac{\beta_p}{4}p^4 + \frac{\kappa_p}{2}(\partial_\alpha p_\beta)(\partial_\alpha p_\beta)\right] \tag{S.4}$$

$$f_Q = \rho^2\left[-\frac{\alpha_Q}{2}\frac{\rho}{\rho_0}Q^2 + \frac{\beta_Q}{2}Q^4 + \frac{\kappa_Q}{2}(\partial_\alpha Q_{\beta\gamma})(\partial_\alpha Q_{\beta\gamma})\right] \tag{S.5}$$

$$f_{pQ} = -\frac{\chi}{2}\rho^2 Q_{\alpha\beta}\left(p_\alpha p_\beta - \frac{p_\gamma p_\gamma}{2}\delta_{\alpha\beta}\right) = \frac{\chi}{2}\rho^2\left[Q_1(p_y^2 - p_x^2) - 2Q_2 p_x p_y\right]\ . \tag{S.6}$$

Here, we defined $p^2 \equiv p_\gamma p_\gamma$, $p^4 \equiv (p^2)^2$, $Q^2 \equiv \mathrm{Tr}(Q^2) = 2(Q_1^2 + Q_2^2)$, and $Q^4 \equiv (Q^2)^2$. Inspired by the actomyosin cortex [1], the polar, nematic, and nematopolar components $f_p$, $f_Q$, and $f_{pQ}$ of the free energy density are all scaled with $\rho^2$, so that the corresponding energetic cost is larger when more material is present. The coupling $\chi > 0$ favors local alignment between the polar and nematic fields. Note that making the $p_\alpha p_\beta$ tensor traceless does not affect the coupling term. In a homogeneous system at density $\rho = \rho_0$ and without nematopolar coupling ($\chi = 0$), the polar and nematic fields respectively relax to $p_0^2 = \frac{\alpha_p}{\beta_p}$ and $Q_0^2 = \frac{\alpha_Q}{2\beta_Q}$ and hence $S_0^2 = \frac{\alpha_Q}{\beta_Q}$.

Thermodynamic fields conjugate to the density, orientational order, and surface are obtained by taking the corresponding derivatives of the free energy. Explicitly:

- Chemical potential: $\mu = \frac{\delta F}{\delta\rho}$ yields $\mu = \mu_c + \mu_p + \mu_Q + \mu_{pQ}$ with

$$\mu_c = a\rho^3 \tag{S.7}$$

$$\mu_p = -\frac{3\alpha_p}{2\rho_0}\rho^2 p^2 + \rho\left[\frac{\beta_p}{2}p^4 + \kappa_p(\partial_\alpha p_\beta)(\partial_\alpha p_\beta)\right] \tag{S.8}$$

$$\mu_Q = -\frac{3\alpha_Q}{2\rho_0}\rho^2 Q^2 + \rho\left[\beta_Q Q^4 + \kappa_Q(\partial_\alpha Q_{\beta\gamma})(\partial_\alpha Q_{\beta\gamma})\right] \tag{S.9}$$

$$\mu_{pQ} = -\rho\chi Q_{\alpha\beta}\left(p_\alpha p_\beta - \frac{p_\gamma p_\gamma}{2}\delta_{\alpha\beta}\right) = \rho\chi\left[Q_1(p_y^2 - p_x^2) - 2Q_2 p_x p_y\right]\ . \tag{S.10}$$

- Polar molecular field: $h_\alpha = -\frac{\delta F}{\delta p_\alpha}$ yields $h_\alpha = h_\alpha^p + h_\alpha^{pQ}$ with

$$h_\alpha^p = -\rho^2\left(\beta_p p^2 - \alpha_p\frac{\rho}{\rho_0}\right)p_\alpha + 2\kappa_p\rho\partial_\beta\rho\partial_\beta p_\alpha + \kappa_p\rho^2\partial_\beta\partial_\beta p_\alpha \tag{S.11}$$

$$h_\alpha^{pQ} = \rho^2\chi Q_{\alpha\gamma}p_\gamma\ . \tag{S.12}$$

- Nematic molecular field: $H_\alpha = -\frac{\delta F}{\delta Q_\alpha}$ yields $H_\alpha = H_\alpha^Q + H_\alpha^{pQ}$ for $\alpha \in \{1,2\}$ with

$$H_\alpha^Q = -2\rho^2 \left(2\beta_Q Q^2 - \alpha_Q \frac{\rho}{\rho_0}\right) Q_\alpha + 4\kappa_Q \rho \partial_\beta \rho \partial_\beta Q_\alpha + 2\kappa_Q \rho^2 \partial_\beta \partial_\beta Q_\alpha \tag{S.13}$$

$$H_1^{pQ} = \frac{\rho^2}{2}\chi(p_x^2 - p_y^2) \tag{S.14}$$

$$H_2^{pQ} = \rho^2 \chi p_x p_y \; . \tag{S.15}$$

- Hydrostatic pressure: $\Pi = \rho\mu - f$ yields

$$\Pi = \frac{3}{4}a\rho^4 + \rho^2 \left[-\alpha_p \frac{\rho}{\rho_0} p^2 + \frac{\beta_p}{4} p^4 + \frac{\kappa_p}{2} \partial_\alpha p_\beta \partial_\alpha p_\beta - \alpha_Q \frac{\rho}{\rho_0} Q^2 + \frac{\beta_Q}{2} Q^4 + \frac{\kappa_Q}{2} \partial_\alpha Q_{\beta\gamma} \partial_\alpha Q_{\beta\gamma} - \frac{\chi}{2} Q_{\alpha\beta} p_\alpha p_\beta \right] . \tag{S.16}$$

- Symmetric Ericksen stress: $\sigma^{\mathrm{e,s}}_{\alpha\beta} = -\Pi\delta_{\alpha\beta} - \frac{\partial f}{\partial(\partial_\beta p_\gamma)}\partial_\alpha p_\gamma - \frac{\partial f}{\partial(\partial_\beta Q_{\gamma\delta})}\partial_\alpha Q_{\gamma\delta}$, where

$$-\frac{\partial f}{\partial(\partial_\beta p_\gamma)}\partial_\alpha p_\gamma = -\kappa_p \rho^2 \partial_\beta p_\gamma \partial_\alpha p_\gamma \tag{S.17}$$

$$-\frac{\partial f}{\partial(\partial_\beta Q_{\gamma\delta})}\partial_\alpha Q_{\gamma\delta} = -\kappa_Q \rho^2 \partial_\beta Q_{\gamma\delta} \partial_\alpha Q_{\gamma\delta} = -2\kappa_Q \rho^2 \partial_\beta Q_\epsilon \partial_\alpha Q_\epsilon \tag{S.18}$$

  with $\epsilon \in \{1,2\}$.

- Anti-symmetric Ericksen stress: $\sigma^{\mathrm{e,a}}_{\alpha\beta} = \frac{1}{2}(p_\alpha h_\beta - p_\beta h_\alpha) + (Q_{\alpha\gamma} H_{\gamma\beta} - H_{\alpha\gamma} Q_{\gamma\beta})$. The only independent component in $2d$ is the off-diagonal one, which we express as

$$\sigma^{\mathrm{e,a}}_{xy} = \frac{1}{2}(p_x h_y - p_x h_y) + 2(Q_1 H_2 - H_1 Q_2) \; . \tag{S.19}$$

Having defined the equilibrium thermodynamic quantities, we use nonequilibrium thermodynamics to derive the hydrodynamic equations for the active nematopolar fluid [1–4]. The resulting equations generalize standard active-gel theory equations and accounts for both, nematic and polar order fields, as well as material renewal. Finally, we consider the overdamped limit of the force-balance equation in the presence of friction. All in all, the non-dimensionalized hydrodynamics equations read

$$\partial_t \rho = -\partial_\beta (v_\beta \rho - D\partial_\beta \rho) + \tau^{-1}(\rho_0 - \rho) \tag{S.20}$$

$$v_\alpha = \partial_\beta \sigma_{\alpha\beta} \tag{S.21}$$

$$\sigma_{\alpha\beta} = 2v_{\alpha\beta} + \frac{\nu}{2}(p_\alpha h_\beta + p_\beta h_\alpha) + \bar{\nu} p_\gamma h_\gamma \delta_{\alpha\beta} + 2\lambda H_{\alpha\beta} + \sigma^{\mathrm{e,a}}_{\alpha\beta} + \sigma^{\mathrm{e,s}}_{\alpha\beta} - \zeta_Q \rho Q_{\alpha\beta} \tag{S.22}$$

$$h_\alpha = -\rho^2 \left(\beta_p p^2 - \alpha_p \frac{\rho}{\rho_0}\right) p_\alpha + \kappa_p \partial_\beta (\rho^2 \partial_\beta p_\alpha) + \rho^2 \chi Q_{\alpha\gamma} p_\gamma \tag{S.23}$$

$$H_{\alpha\beta} = -2\rho^2 \left(2\beta_Q Q^2 - \alpha_Q \frac{\rho}{\rho_0}\right) Q_{\alpha\beta} + 2\kappa_Q \partial_\gamma (\rho^2 \partial_\gamma Q_{\alpha\beta}) + \delta_{\alpha\beta}\rho^2 \frac{\chi}{2}(p_x^2 - p_y^2) + (1 - \delta_{\alpha\beta})\rho^2 \chi p_x p_y \tag{S.24}$$

$$\partial_t p_\alpha = -v_\gamma \partial_\gamma p_\alpha - \Omega_{\alpha\gamma} p_\gamma + \Gamma_p^{-1} h_\alpha - \nu p_\beta v_{\alpha\beta} - \bar{\nu} p_\alpha v_{\gamma\gamma} \tag{S.25}$$

$$\partial_t Q_{\alpha\beta} = -v_\gamma \partial_\gamma Q_{\alpha\beta} - \Omega_{\alpha\gamma} Q_{\gamma\beta} + \Gamma_Q^{-1} H_{\alpha\beta} - 2\lambda \left(v_{\alpha\beta} - \frac{1}{2} v_{\gamma\gamma}\right) \; . \tag{S.26}$$

In our study, we do not consider flow-alignment, $\nu = \bar{\nu} = \lambda = 0$, and set $\alpha_p = 0$, $\beta_p \equiv \beta$, and $\alpha_Q = \beta_Q \equiv \alpha$. Furthermore, we set $\Gamma_p = \Gamma_Q = 1$.

## SII. Numerical solution of the dynamic equations

In this section, we give details for numerical integration of the dynamic Eqs. (S.20)-(S.26).

### A. Integration scheme

Spatial derivatives were calculated by first transforming the dynamic fields to reciprocal space using the Fast Fourier Transform (FFT), then multiplying with the corresponding wave vectors and, finally, transforming back to real space using FFT. Temporal integration was executed through the explicit forward Euler scheme. We solved the equations on a grid of at least $512 \times 512$ points, with spatial discretization $\Delta x = L/N$. The maximal time step is set to $\Delta t_{\max} = 10^{-2}$ and the actual time step $\Delta t$ is chosen at every time unit according to $\Delta t = \min\left\{\Delta t_{\max},\, 5 \cdot 10^{-2}\Delta x/\max\left(||v||\right),\, 1.25\Delta t_{\mathrm{prev}}\right\}$ with $\Delta t_{\mathrm{prev}}$ being the previous time step. The computations were performed on GPUs using Julia and CUDA.jl [5, 6].

At each time step, first, the chemical potential $\mu$, the molecular fields $h_\alpha$ and $H_\alpha$, and the non-viscous stress $\sigma^{\mathrm{nv}}_{\alpha\beta} = \sigma^{\mathrm{tot}}_{\alpha\beta} - (\partial_\alpha v_\beta + \partial_\beta v_\alpha)$, were computed in real space. Then, the velocity field was computed by solving the force balance equation in Fourier space:

$$(1 + 2k_x^2 + k_y^2)\hat{v}_x + k_x k_y \hat{v}_y = i(k_x \hat{\sigma}^{\mathrm{nv}}_{xx} + k_y \hat{\sigma}^{\mathrm{nv}}_{xy}) \tag{S.27}$$

$$(1 + 2k_y^2 + k_x^2)\hat{v}_y + k_y k_x \hat{v}_x = i(k_y \hat{\sigma}^{\mathrm{nv}}_{yy} + k_x \hat{\sigma}^{\mathrm{nv}}_{yx})\ , \tag{S.28}$$

which yields

$$\hat{v}_y = \frac{i}{k_x^2 + 2k_y^2 + 1 - \frac{k_y^2 k_x^2}{k_y^2 + 2k_x^2 + 1}} \left[ k_y \hat{\sigma}^{\mathrm{nv}}_{yy} + k_x \hat{\sigma}^{\mathrm{nv}}_{yx} - \frac{k_x k_y (k_y \hat{\sigma}^{\mathrm{nv}}_{xy} + k_x \hat{\sigma}^{\mathrm{nv}}_{xx})}{k_y^2 + 2k_x^2 + \xi} \right]\ , \tag{S.29}$$

$$\hat{v}_x = \frac{i(k_y \hat{\sigma}^{\mathrm{nv}}_{xy} + k_x \hat{\sigma}^{\mathrm{nv}}_{xx}) - k_x k_y \hat{v}_y}{k_y^2 + 2k_x^2 + 1}\ . \tag{S.30}$$

Finally, the density, nematic and polarity fields were updated.

All simulations are performed for a minimum time of $T = 10^5$. Simulations of Fig. 1d to obtain the string length are performed until convergence of $\ell$ in time, with a minimum time of $T \geq 3 \times 10^5$.

### B. Initial conditions

Here, we list the different initial conditions employed in our simulations:

- Disordered: $\mathbf{p}$, Q are set to 0; $\rho$ is set to $\rho_0$; zero-average noise is added to each grid point for the three fields. Used for Fig. 1a,b and Fig. 4.

- Polarized along $\hat{x}$: $p = p^\star$, $S = S^\star$, $\nu = \psi = 0$; $\rho$ is set to $\rho_0$; zero-average noise is added to each grid point for the three fields. Used for Fig. 5a.

- Loop: we initialize a ring of radius $R$ and width $w$, corresponding to the polar defect, centered at $(L/2, L/2)$. At distances $r < R - w/2$ from the centre, we set $\mathbf{p} = p^\star \hat{x}$; for $r > R + w/2$, $\mathbf{p} = -p^\star \hat{x}$. In the defect region $R - w/2 < r < R + w/2$, we vary $p$ smoothly from $p^\star$ to $-p^\star$. The nematic order is $S = S^\star$ everywhere and the nematic director points along $\hat{x}$. $\rho$ is set to $\rho_0$; zero-average noise is added to each grid point for the three fields. Used for Fig. 1c.

- 4-string lattice: an arrangement of 4 topological strings, two with negative, two with positive charge as depicted in Fig. S2. The density field is scaled so that the average density is $\rho_0$. Since negative strings, when too long, are susceptible to the transverse instability described in the main text, we adapt the initial length to the value of $\chi$ (compare Fig. S2a-c to Fig. S2d-f). Used for Fig. 1d, Fig. 2, Fig. 3.

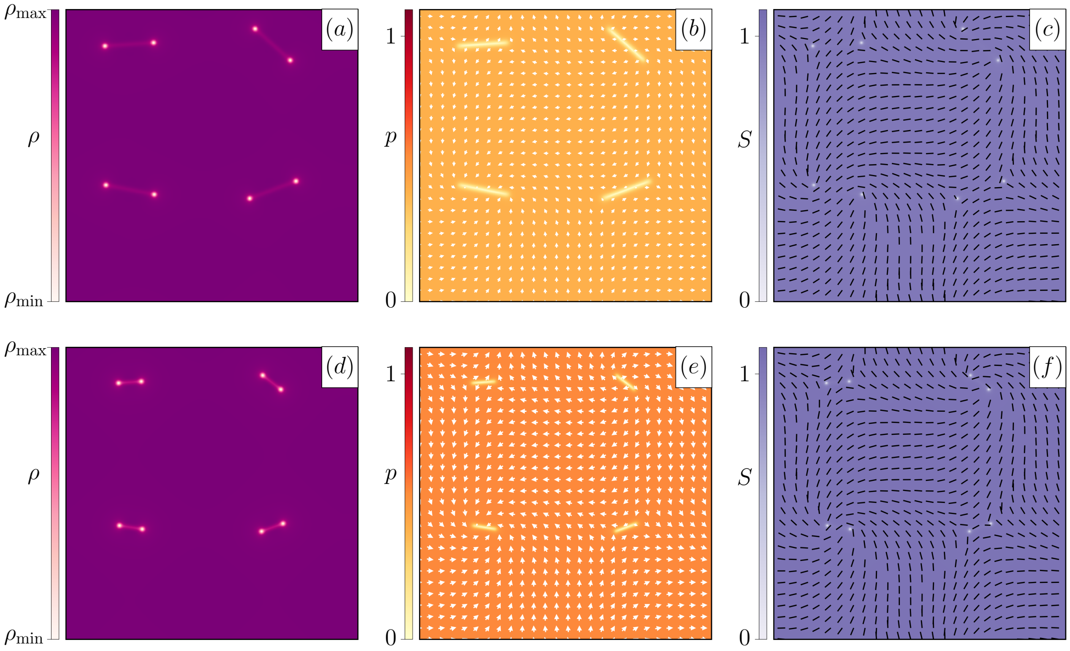


FIG. S2. Examples of initial condition with 4 strings organized into a square lattice (density, polar and nematic field are respectively shown), with $N = 2048$ lattice points. In Fig. 1d, initial conditions (a-c) are used for $\chi \leq 0.11$, while (d-f) are used for $\chi > 0.11$.

### C. Data analysis

To analyze the numerical solutions, we developed a Julia scriptwhich relies on the Julia package `Image.jl`. To identify the strings, we first apply a mask based on the local value of $p$, where the threshold is set to $p < 0.5\, p_{\max}$ with $p_{\max}$ being the maximal value for $p$ measured in at a given time. String lengths are obtained by skeletonizing the masked region and determining the length of the corresponding skeleton. We estimate a relative uncertainty of 10% to our length measurements obtained with this method. Profiles of density, velocity, forces and pressure are obtained along the skeleton. Vectorial quantities are projected along the string axis.

## SIII. Equilibrium behavior of nematopolar systems

In this section, we discuss the equilibrium behavior of the system described by the free energy of Eqs. (S.2)–(S.6), and derive the equilibrium scaling for the string length as a function of the nematopolar coupling $\chi$. In order to keep the expressions tractable, we first express the coupling term in terms of the order parameters $S$ and $p$ and the angles $\psi$ and $\nu$, where $\hat{n} = (\cos\psi, \sin\psi)$ and $\hat{p} = (\cos\nu, \sin\nu)$. This yields

$$Q_{\alpha\beta} p_\alpha p_\beta = Sp^2 \left( \hat{n}_\alpha \hat{n}_\beta \hat{p}_\alpha \hat{p}_\beta - \frac{1}{2} \delta_{\alpha\beta} \hat{p}_\alpha \hat{p}_\beta \right) = Sp^2 \left[ (\hat{n} \cdot \hat{p})^2 - 1/2 \right] = \frac{Sp^2}{2} \cos[2(\psi - \nu)] \; . \tag{S.31}$$

Hence, the coupling term can be expressed as

$$f_{pQ} = -\chi \frac{Sp^2}{4} \cos[2(\psi - \nu)] \; . \tag{S.32}$$

When $\chi > 0$, the coupling favors alignment between the polar and nematic directors. In order to determine configurations of minimal energy, we thus take $\psi = \nu$ at all points in space. As in the main text, we consider the case where the polar field has tendency to disorder by setting $\alpha_p = 0$ and $\beta_p > 0$. Note that our choice corresponds to having a critical (massless) $p$-field in the uncoupled regime, $\chi = 0$.

### A. Homogeneous and distortion-free configurations

Before discussing the properties of topological string defects, it is useful to characterize the minimal-energy states of a homogeneous, distortion-free configuration. The corresponding free-energy density is given by

$$f = -\frac{\alpha}{4}S^2 + \frac{\alpha}{8}S^4 + \frac{\beta}{4}p^4 - \chi\frac{Sp^2}{4} \ , \tag{S.33}$$

where we have assumed $\alpha_Q = \beta_Q \equiv \alpha$, $\beta_p = \beta$, and $\alpha_p = 0$ as in the main text. Minimization of $f$ with respect to $S$ and $p$ yields

$$-\alpha S + \alpha S^3 = \chi\frac{p^2}{2} \tag{S.34}$$

$$p(\beta p^2 - \frac{\chi}{2}S) = 0 \ . \tag{S.35}$$

In the presence of nematopolar coupling $\chi \neq 0$, the local extreme at $S_0 = 1, p_0 = 0$ is destabilized in favor of a new global minimum

$$S^\star = \sqrt{1 + \frac{\chi^2}{4\alpha\beta}} \tag{S.36}$$

$$p^\star = \sqrt{\frac{|\chi|}{2\beta}S^\star} \ . \tag{S.37}$$

The difference $\Delta$ between the energy density of configurations $(S, p) = (1, 0)$ and $(S^\star, p^\star)$ is

$$\Delta = \frac{\chi^2\left[8\alpha\beta + \chi^2\right]}{128\beta^2\alpha} \simeq \frac{\chi^2}{16\beta}S_0^2 \sim \chi^2 \tag{S.38}$$

to leading order in $\chi$. As expected, the stronger the coupling, the higher the energetic cost associated with the local minimum at $(1, 0)$.

To estimate the width of topological strings, we compute the correlation length associated with the polar field. We To estimate the correlation length close associated to the minimal energy configuration $(S^\star, p^\star)$, we compute the associated Hessian of the free energy. It reads

$$H = \begin{pmatrix} -\frac{\alpha}{2} + \frac{3}{2}\alpha(S^\star)^2 & -\frac{\chi}{2}p^\star \\ -\frac{\chi}{2}p^\star & \chi S^\star \end{pmatrix} \ . \tag{S.39}$$

The Hessian is non-diagonal, meaning that the eigendirections associated with the local Gaussian theory around the minimum are combinations of $p, S$. However, we remark that the off-diagonal terms are at least of order $|\chi|^{3/2}$, while diagonal terms are respectively of order $S_0^2 \sim \mathcal{O}(1)$ and $\mathcal{O}(\chi)$. To estimate the correlation length of the polar field close to the minimum we thus take $H_{22}$ to be the mass of the polar field, and $\kappa_p$ its elastic constant, thus obtaining

$$\xi_p \simeq \sqrt{\frac{\kappa_p}{H_{22}}} = \sqrt{\frac{\kappa_p}{\chi S^\star}} \sim \chi^{-1/2} \ . \tag{S.40}$$

As expected, the correlation length of the polar field diverges as we approach the critical point for $\chi = 0$. In the following we do not focus on the critical behavior of our system and work sufficiently far from the critical point, meaning that $\xi_p \ll L$, where $L$ is the system size.

### B. Topological constraints and string-length selection.

Unless enforced by the boundary conditions, there are no defects at equilibrium. However, topological strings that are sufficiently far away from other defects will persist for some time in a configuration that is determined by the free energy. We now consider such topological strings at equilibrium.

When two nematic defects form, the coupling term $\mathcal{F}_{pQ}$ imposes a topological constraint on the polar field. To see this, let us define by $q_1, q_2$ the nematic charges associated with the two nematic defects. By integrating the nematic field around the pair of defects we obtain:

$$\oint_C \phi(\theta)\mathrm{d}\theta = 2\pi(q_1 + q_2) \,. \tag{S.41}$$

For aligning interactions, the coupling energy is minimized when $\psi = \phi$ modulo $\pi$. As a consequence, the polar charge $q_p$ is given by:

$$2\pi q_p = \oint_C \psi(\theta)\mathrm{d}\theta = \oint_C [\phi(\theta) + k\pi]\mathrm{d}\theta = 2\pi(q_1 + q_2) \,, \tag{S.42}$$

where $q_p \in \mathbb{Z}$, $q_{1,2} \in \frac{1}{2}\mathbb{Z}$. In other words, the presence of two nematic defects induces, via the coupling term, a defect in the polar field with total charge:

$$q_p = q_1 + q_2 \,. \tag{S.43}$$

We note that the polar defects generated by such coupling must necessarily connect two half-integer nematic defects. If this were not the case, then the topological charge associated with $\psi$ around the nematic charge would be half-integer, which is not admissible for the polar field. Hence, a pair of nematic defects induces the formation of polar-defect strings connecting the two nematic defects.

Following the reasoning of Ref. [7], we now compute the length of topological strings and determine which forces act on a straight defect line of length $\ell$ and width $w \sim \xi_p$. The interaction between nematic charges results in a Coulomb force $f_c(\ell) = 2\pi\kappa_Q q_1 q_2/\ell$, which is repulsive for charges of equal sign. Meanwhile, the energetic cost of creating an extended region with $(S, p) = (1, 0)$ generates an effective tension $T = w\Delta$. Using Eqs. (S.38) and (S.40), balancing the Coulomb force with the line tension leads to

$$\ell = \frac{\pi\kappa_Q}{2\xi_p(\chi)\Delta(\chi)} \sim \chi^{-3/2} \tag{S.44}$$

for $q_1 = q_2 = \pm 1/2$. Crucially, there is no difference between positively and negatively charged strings. On a final note, we remark that strings with zero charge are always unstable and self-annihilate in this equilibrium setting, since both, tension and Coulomb force, are attractive. This also holds for loop configurations.

In order to test relation (S.44) between the string length and $\chi$, we obtained the length of strings in the equilibrium setting from our numerical solutions. We initialize the system in the 4-string lattice configuration where the strings are sufficiently far apart, so that Coulomb interactions between different strings are negligible during the simulations. We find good agreement between our numerical and analytical results, Fig. S3.

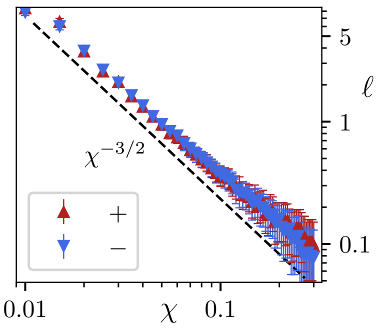


FIG. S3. String length in the absence of renewal for topological strings of positive (red) and negative (blue) charge. Parameters as in Fig. 1d of the main text, except for the renewal rate: $\rho_0 = 0.6$, and $\tau^{-1} = 0$. Simulations are performed with $L = 10, N = 1024$ for $\chi > 0.03$ and $L = 20, N = 2048$ for $\chi \leq 0.03$, with initial conditions corresponding to Fig. S2a-c.

## SIV. Mechanical properties of active nematopolar fluids with renewal

In this Section we compute the hydrodynamic pressure, anti-symmetric Ericksen stress tensor, and compressibility of a nematopolar fluid, to derive Eqs. (7-9) of the main text.

### A. Hydrostatic pressure associated with topological point defects

We consider a homogeneous system at $\rho = \rho_0$ and compute the corresponding hydrostatic pressure $\Pi$, Eq. (S.16), in the bulk of the system and for nematic and polar defects. We express the pressure as a function of the order parameters $S$ and $p$, where we neglect the contributions from the Frank free energy:

$$\Pi = \frac{3}{4}a\rho^4 + \rho^2\left[\frac{\beta}{4}p^4 - \frac{\alpha}{2}\frac{\rho}{\rho_0}S^2 + \frac{\alpha}{8}S^4 - \frac{\chi}{4}Sp^2\right] . \tag{S.45}$$

We then compute the pressure in different regions assuming that $\rho = \rho_0$ everywhere. Consequently, the term in $\Pi$ proportional to $a$ is constant throughout the system and can be neglected in what follows. In defect-free regions, we find

$$\Pi_0 = -\rho_0^2\alpha\frac{(\chi^2+4\alpha\beta)(\chi^2+12\alpha\beta)}{128\beta^2\alpha^2} = -\frac{3}{8}\rho_0^2\alpha\left(1+\frac{\chi^2}{4\alpha\beta}\right)\left(1+\frac{\chi^2}{12\alpha\beta}\right) . \tag{S.46}$$

For a nematic defect core, that is, at the extremes of a string, $p = S = 0$, so that the pressure is

$$\Pi_{\rm Q} = 0 . \tag{S.47}$$

Finally, along a string, $p = 0$ and $S \simeq 1$, so that

$$\Pi_{\rm p} = -\frac{3}{8}\alpha\rho_0^2 . \tag{S.48}$$

By taking the difference between the distinct contributions, $\Delta\Pi^{\rm e}_{\rm out} = \Pi_{\rm Q} - \Pi_0$ and $\Delta\Pi^{\rm e}_{\rm in} = \Pi_{\rm Q} - \Pi_{\rm p}$ we obtain the pressure differences reported in Eq. (7) of the main text.

### B. Anti-symmetric Ericksen stress

In this subsection, we give an explicit expression for the anti-symmetric part of the Ericksen stress tensor $\sigma^{\rm e,a}_{xy} = \frac{1}{2}(p_xh_y - p_yh_x) + 2(Q_1H_2 - H_1Q_2)$. We show that it consists of three contributions: two elastic terms $\sigma^{\rm el}_{\rm p}$ and $\sigma^{\rm e,a}_{\rm Q}$, and a nematopolar bulk contribution $\sigma^{\rm mis}$ resulting from misalignment between the polar and nematic fields. The elastic polar terms is

$$\sigma^{\rm e,a}_{\rm p} = \frac{\kappa_p}{2}[p_x\partial_\gamma(\rho^2\partial_\gamma p_y) - p_y\partial_\gamma(\rho^2\partial_\gamma p_x)] \tag{S.49}$$

$$= \frac{\kappa_p}{2}\mathbf{p}\times\partial_\gamma(\rho^2\partial_\gamma\mathbf{p}) . \tag{S.50}$$

To understand the role of this term close to the extremes of the string, we take the approximation of constant density $\rho \simeq \rho_0$. We then decompose the polar field as $p_x = p\cos\nu$, $p_y = p\sin\nu$ and write:

$$p_x\nabla^2p_y = p\cos\nu\nabla^2[p\sin\nu] \tag{S.51}$$

$$= p\cos\nu[\sin\nu\nabla^2p + 2\cos\nu\nabla p\cdot\nabla\nu + p\nabla^2\sin\nu] \tag{S.52}$$

$$= p\cos\nu[\sin\nu\nabla^2p + 2\cos\nu\nabla p\cdot\nabla\nu - p\sin\nu(\nabla\nu)^2 + p\cos\nu\nabla^2\nu] \tag{S.53}$$

$$= p\cos\nu\sin\nu\nabla^2p + 2\cos^2\nu p\nabla p\cdot\nabla\nu - p^2\cos\nu\sin\nu(\nabla\nu)^2 + p^2\cos^2\nu\nabla^2\nu \tag{S.54}$$

and

$$p_y\nabla^2p_x = p\sin\nu\nabla^2[p\cos\nu] \tag{S.55}$$

$$= p\sin\nu[\cos\nu\nabla^2p - 2\sin\nu\nabla p\cdot\nabla\nu + p\nabla^2\cos\nu] \tag{S.56}$$

$$= p\cos\nu\sin\nu\nabla^2p - 2\sin^2\nu p\nabla p\cdot\nabla\nu - p^2\cos\nu\sin\nu(\nabla\nu)^2 - p^2\sin^2\nu\nabla^2\nu . \tag{S.57}$$

We thus get

$$\sigma^{\rm e,a}_{\rm p} \simeq \frac{\kappa_p}{2}\rho_0^2[p_x\nabla^2p_y - p_y\nabla^2p_x] \tag{S.58}$$

$$= \frac{\kappa_p}{2}\rho_0^2\left[\nabla p^2\cdot\nabla\nu + p^2\nabla^2\nu\right] . \tag{S.59}$$

Similarly, the elastic nematic term can be written as

$$\sigma_{\rm Q}^{\rm e,a} = 2\kappa_Q[Q_1\partial_\gamma(\rho^2\partial_\gamma Q_2) - Q_2\partial_\gamma(\rho^2\partial_\gamma Q_1)] \ . \tag{S.60}$$

With $Q_1 = \frac{S}{2}\cos(2\psi)$, $Q_2 = \frac{S}{2}\sin(2\psi)$ we eventually obtain

$$\sigma_{\rm Q}^{\rm e,a} \simeq 2\kappa_Q\rho_0^2[Q_1\nabla^2 Q_2 - Q_2\nabla^2 Q_1] \tag{S.61}$$

$$= \kappa_Q\rho_0^2\left[\nabla S^2\cdot\nabla\psi + S^2\nabla^2\psi\right] \ . \tag{S.62}$$

We now turn to the misalignment term $\sigma^{\rm mis}$ which directly results from the nematopolar coupling. This reads:

$$\sigma^{\rm mis} = \frac{1}{2}\rho^2\chi(p_xQ_{yx}p_x + p_xQ_{yy}p_y - p_yQ_{xx}p_x - p_yQ_{xy}p_y) + 2\rho^2\chi\left[Q_{xx}p_xp_y - \frac{1}{2}Q_{xy}(p_x^2 - p_y^2)\right] \tag{S.63}$$

$$= \frac{1}{2}\rho^2\chi\left[Q_{xy}p_x^2 - Q_{xx}p_xp_y - Q_{xx}p_xp_y - Q_{xy}p_y^2 + 4Q_{xx}p_xp_y - 2Q_{xy}p_x^2 + 2Q_{xy}p_y^2\right] \tag{S.64}$$

$$= \frac{1}{2}\rho^2\chi\left[Q_{xy}(p_y^2 - p_x^2) + 2Q_{xx}p_xp_y\right] \tag{S.65}$$

$$\equiv \frac{1}{2}\rho^2\chi\left[Q_2(p_y^2 - p_x^2) + 2Q_1p_xp_y\right] \ . \tag{S.66}$$

In terms of the order parameters $p$ and $S$ and the director angles $\nu$ and $\psi$, Eq. (S.66) can be written as

$$\sigma^{\rm mis} = \rho^2\chi\frac{Sp^2}{4}[\sin(2\psi)(\sin^2\nu - \cos^2\nu) + 2\cos(2\psi)\sin\nu\cos\nu] \tag{S.67}$$

$$= \rho^2\chi\frac{Sp}{2}[-\sin(2\psi)\cos(2\nu) + \cos(2\psi)\sin(2\nu)] \tag{S.68}$$

$$= \rho^2\chi\frac{Sp^2}{4}\sin\left[2(\nu-\psi)\right] \ . \tag{S.69}$$

Consequently, misalingment between the two director angles induces an additional contribution to the anti-symmetric stress tensor. As reported in Fig. S4, the misalignment contribution dominates over the elastic one in the presence of renewal.

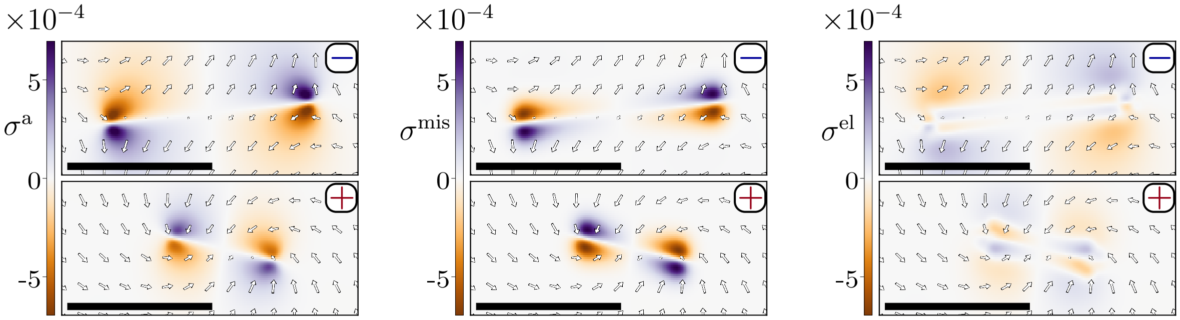


FIG. S4. Heatmaps of the components of the antisymmetric stress $\sigma_{\rm xy}^{\rm a}$ in the presence of renewal, for positive and negative strings. (**a**) Total antisymmetric stress. (**b**) Misalignment antisymmetric stress $\sigma^{\rm mis}$. (**c**) Elastic antisymmetric stress $\sigma^{\rm el}$. We use the same parameters as in Fig. 3a-b of the main text: $\rho_0 = 0.6$, $\tau^{-1} = 5$, and $\chi = 0.1$ .

## C. Bulk compressibility and conditions for mechanical stability

In this section, we compute the bulk modulus $K$ at density $\rho$, which is given by

$$K(\rho) = \rho\frac{d\Pi}{d\rho} = \rho^2\frac{d\mu}{d\rho} \ , \tag{S.70}$$

and determine the conditions under which $K(\rho) > 0$. In this case, the homogeneous density field is mechanically stable at equilibrium. Respecting this inequality is crucial for initializing the numerical solutions in conditions that allow us to compare them to the analytical expressions derived above.

For the calculation, we assume that $p_\alpha, Q_{\alpha\beta}$ have relaxed locally to the minima of the free energy, so that the respective director fields are aligned and the scalar order parameters have reached the global minimum $(p^\star, S^\star)$. For a homogeneous system at density $\rho = \rho_0$, we then find

$$K(\rho) = 3a\rho^4 \left(1 - \frac{g(\chi)}{\rho^2}\right) , \tag{S.71}$$

where

$$g(\chi) = \frac{1}{3a}\left[-\frac{\beta}{2}(p^\star)^4 + 3\alpha(S^\star)^2 - \frac{\alpha}{2}(S^\star)^4 + \frac{\chi}{2}S^\star(p^\star)^2\right] . \tag{S.72}$$

Depending on the sign of the factor $1 - g(\chi)/\rho^2$, the system is either mechanically stable (positive $K$) or unstable. Stability thus requires that the density is sufficiently large, $\rho > \sqrt{g(\chi)}$.

## SV. Green function for Brinkmann-Darcy flow

In this section, we derive explicitly the Green function associated to the Brinkmann-Darcy flow $v(\mathbf{r})$. It is convenient to work in dimensional units and to retrieve the case studied in the main text upon setting $\xi = \eta = 1$. We consider the linear operator$\mathcal{L}$ acting on the velocity field $\mathbf{v}(\mathbf{r})$ with

$$\mathcal{L}_{\alpha\beta} v_\beta = \xi\, v_\alpha - \eta\, \partial_\gamma \left(\partial_\alpha v_\gamma + \partial_\gamma v_\alpha\right) \tag{S.73}$$

and define the propagator $G_{\alpha\beta}(\mathbf{r})$ as

$$\mathcal{L}_{\alpha\gamma} G_{\gamma\beta}(\mathbf{r}) = \delta_{\alpha\beta}\, \delta(\mathbf{r}). \tag{S.74}$$

Following a Fourier transform, $\partial_\alpha \to ik_\alpha$ and the operator becomes

$$\mathcal{L}_{\alpha\beta}(\mathbf{k}) = \left(\xi + \eta k^2\right) \delta_{\alpha\beta} + \eta\, k_\alpha k_\beta , \tag{S.75}$$

where $k^2 = k_\gamma k_\gamma$. We introduce the longitudinal and transverse projectors $P^L_{\alpha\beta} = k_\alpha k_\beta / k^2$ and $P^T_{\alpha\beta} = \delta_{\alpha\beta} - P^L_{\alpha\beta}$, to express the operator $\mathcal{L}_{\alpha\beta}$ as

$$\mathcal{L}(\mathbf{k}) = \left(\xi + \eta k^2\right) P^T + \left(\xi + 2\eta k^2\right) P^L. \tag{S.76}$$

In Fourier space, the Green function is therefore

$$\tilde{G}_{\alpha\beta}(\mathbf{k}) = \frac{1}{\xi}\left(\delta_{\alpha\beta} - \frac{k_\alpha k_\beta}{k^2}\right)\frac{1}{1 + \ell_T^2 k^2} + \frac{1}{\xi}\frac{k_\alpha k_\beta}{k^2}\frac{1}{1 + \ell_L^2 k^2} , \tag{S.77}$$

where we have introduced the transverse and longitudinal screening lengths $\ell_T^2 = \eta/\xi$ and $\ell_L^2 = 2\eta/\xi$. After applying the inverse Fourier transform, the real-space propagator reads

$$G_{\alpha\beta}(\mathbf{r}) = A(r)\, \delta_{\alpha\beta} + B(r)\, \frac{r_\alpha r_\beta}{r^2} \tag{S.78}$$

with scalar functions

$$A(r) = \frac{1}{4\pi\eta}\left[K_0\left(\frac{r}{\ell_T}\right) - K_0\left(\frac{r}{\ell_L}\right)\right] \tag{S.79}$$

and

$$B(r) = \frac{1}{4\pi\eta}\left[K_0\left(\frac{r}{\ell_L}\right) - K_0\left(\frac{r}{\ell_T}\right) + \frac{r}{\ell_L}K_1\left(\frac{r}{\ell_L}\right) - \frac{r}{\ell_T}K_1\left(\frac{r}{\ell_T}\right)\right]. \tag{S.80}$$

Here, $K_0$, $K_1$ are the modified Bessel functions of the zeroth and first type, respectively. The term proportional to $\delta_{\alpha\beta}$ encodes isotropic response to the force. The second term projects the force along the distance vector $\mathbf{r}$.

## SVI. Hydrodynamic forces and material fluxes

In this section, we analyze the contributions of the various components of the hydrodynamic force to the material flux in the steady state numerical solution presented in Fig. 2 of the main text, Fig. S6. The hydrostatic force $\mathbf{f}^{\mathrm{e}}$ resulting from the effective pressure $\Pi^{\mathrm{e}} = \frac{1}{2}\mathrm{Tr}[\sigma^{\mathrm{e}}]$ via $\mathbf{f}^{\mathrm{e}} = -\boldsymbol{\nabla}\Pi^{\mathrm{e}}$ is amplified by a factor of about 2 due to renewal, Fig. S6a,b,f,g. The contributions resulting from the traceless symmetric part of the Ericksen stress $\sigma^{\mathrm{e,s}}$ hardly differ in the absence and in the presence of renewal, Fig. S6c,h. Also, they are subdominant compared to the contribution from the effective pressure.

The situation is very different for the contribution by the antisymmetric part of the Ericksen stress $\sigma^{\mathrm{a,s}}$, where renewal results in a 10-fold increase compared to the case $\tau^{-1} = 0$, Fig. S6d,i. Furthermore, the contributions to strings with positive and negative topological charges have opposite signs, confirming that it is the only charge-dependent contribution to the stress. Altogether, these forces lead to a material current $\mathbf{J} := \mathbf{v}\rho - D\nabla\rho$ that is two orders of magnitude larger in the presence of renewal compared to case without renewal, Fig. S6e,j.

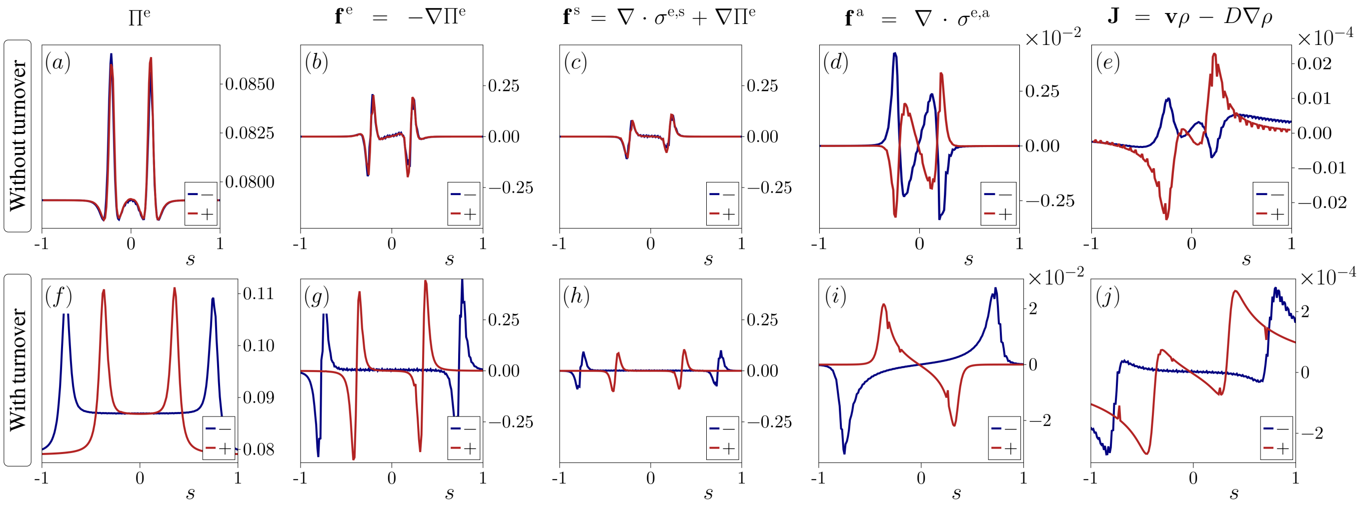


FIG. S6. Hydrodynamic forces and material current for steady state topological strings. All quantities are projected along the string axis. (**a, f**) Effective pressure $\Pi^{\mathrm{e}} = \mathrm{Tr}[\sigma^{\mathrm{e}}]$. (**b, g**) Force resulting from the effective pressure. (**c, h**) Force resulting from the traceless component of the symmetric Ericksen stress. (**d, i**) Force resulting from the antisymmetric component of the Ericksen stress. (**e, j**) Mass current $J_\alpha = \rho v_\alpha - D\partial_\alpha\rho$. Parameter values as Fig. 2 of the main text ($\rho_0 = 0.6,\ \tau^{-1} = 5,\ \chi = 0.1,\ \ L = 20,\ \ N = 2048$), except in panels (a-e) for $\tau^{-1} = 0,\ L = 10,\ N = 1024$ .

## SVII. Linear stability analysis in the presence of activity

In this section, we detail the linear-stability analysis of the homogeneous steady state $(\rho, Q_1, p_x, Q_2, p_y) = (\rho_0, S^\star/2, p^\star, 0, 0)$ of the hydrodynamic equations. We choose to work in dimensional units, so that we are able to see how the instability is affected by the friction coefficient $\xi$.

We consider small perturbations $\delta\mathbf{s} = (\delta\rho, \delta Q_1, \delta p_x, \delta Q_2, \delta p_y)^{\mathrm{t}}$ to the homogeneous steady state. For a perturbation $\delta\mathbf{s}(\mathbf{r}) \propto \exp(i\mathbf{q}\cdot\mathbf{r} + \gamma t)$ with associated wave-vector $\mathbf{q} = q(\cos\theta, \sin\theta)$, we obtain the components of the linearized time-evolution operator using a Mathematica script. We compute its eigenvalues numerically, Fig. 5 in the main text.

Further physical insight into the transition can be gained by considering the case of $\theta = n\pi/2$ with $n = 0, 1$ corresponding to longitudinal and transverse perturbations. In this case, the linear dynamics is characterized by a block matrix:

$$\partial_t \begin{pmatrix} \delta\rho \\ \delta Q_1 \\ \delta p_x \\ \delta Q_2 \\ \delta p_y \end{pmatrix} = \begin{pmatrix} M_{\rho\rho} & M_{\rho Q_1} & M_{\rho p_x} & 0 & 0 \\ M_{Q_1\rho} & M_{Q_1Q_1} & M_{Q_1p_x} & 0 & 0 \\ M_{p_x\rho} & M_{p_xQ_1} & M_{p_xp_x} & 0 & 0 \\ 0 & 0 & 0 & M_{Q_2Q_2} & M_{Q_2p_y} \\ 0 & 0 & 0 & M_{p_yQ_2} & M_{p_yp_y} \end{pmatrix} \begin{pmatrix} \delta\rho \\ \delta Q_1 \\ \delta p_x \\ \delta Q_2 \\ \delta p_y \end{pmatrix} . \tag{S.81}$$

Our numerical analysis showed that the instability occurs in the components $Q_2$ or $p_y$, whereas the other components are linearly stable. We thus consider the $2 \times 2$ block of the matrix associated with $(\delta Q_2, \delta p_y)$. Introducing the factor

$$A(q) = \frac{1}{4\eta} \frac{(q\ell_h)^2}{1+(q\ell_h)^2} , \quad \text{where} \quad \ell_h = \sqrt{\eta/\xi} , \tag{S.82}$$

the components of the block are

$$M_{Q_2Q_2} = \rho_0^2 \left\{ \Gamma^{-1} 2 \Big[ (1-S^2)\alpha - \kappa_Q q^2 \Big] - A(q) \big( 4S^2\kappa_Q q^2 + S\chi p^2 \big) \right\} + (-1)^n 2A(q)\zeta_Q \rho_0 S , \tag{S.83}$$

$$M_{p_yp_y} = \rho_0^2 \left\{ \Gamma^{-1} \Big( -\beta p^2 - \kappa_p q^2 - \frac{1}{2} S\chi \Big) + A(q) p^2 \big( S\chi - \kappa_p q^2 \big) \right\} , \tag{S.84}$$

$$M_{p_yQ_2} = \rho_0^2 \left\{ \Gamma^{-1}\chi p + A(q) \Big( -4\kappa_Q q^2 Sp - \chi p^3 \Big) \right\} + (-1)^n 2A(q)\zeta_Q \rho_0 p , \tag{S.85}$$

$$M_{Q_2p_y} = \rho_0^2 \left\{ \Gamma^{-1}\chi p + A(q)(-\kappa_p q^2 Sp + S^2 p\chi) \right\} . \tag{S.86}$$

Here, we have replaced $S^\star$ by $S$ and $p^\star$ by $p$ to ease notation.

In the limit of $q \to 0$, the prefactor $A(q)$ is finite only if the hydrodynamic length diverges, i.e., for zero friction. For finite friction, $A(q \to 0) = 0$. In that case, the eigenvalues of the $2 \times 2$ block are

$$\gamma_\pm(q=0) = \left\{ 0, -\frac{(p\rho_0)^2}{\Gamma} \left( |\chi| + 2\beta S \right) \right\} , \tag{S.87}$$

which shows that large-scale modes are marginal, such that the active nematopolar transition is of Type II. In the absence of friction, $A(q \to 0) = \eta^{-1}/4$, large-scale modes can be unstable and the resulting instability is of Type III.

## SVIII. Movies

In this section we provide the captions and parameters for all Supplementary Movies.

- **SM Movie 1**: Self-annihilation of topological strings at equilibrium: Heatmap of the polar field $p$. Scale bar: unit length. Same parameters as Fig. 1a except for $\tau^{-1} = 0$.
- **SM Movie 2**: Stabilization and coexistence of topological strings in the presence of renewal: Heatmap of the polar field $p$. Scale bar: unit length. Same parameters as Fig. 1a.
- **SM Movie 3**: Stabilization of topological loops of zero charge in the presence of renewal: Heatmap of the polar field $p$. Scale bar: unit length. Same parameters as Fig. 1c.
- **SM Movie 4**: Wiggling instability for negative topological strings in the presence of renewal: Heatmap of the polar field $p$. Scale bar: unit length. Same parameters as Fig. 3c-d.
- **SM Movie 5**: Spontaneous formation of topological string lattices in the presence of renewal: Heatmap of the polar field $p$. Scale bar: unit length. Same parameters as Fig. 4a.
- **SM Movie 6**: Coexistence between topological loops and string lattices in the presence of renewal: Heatmap of the polar field $p$. Scale bar: unit length. Same parameters as Fig. 4b.
- **SM Movie 7**: Nematopolar chaos in the presence of active stresses, no renewal: Heatmap of the polar field $p$. Scale bar: unit length. Same parameters as Fig. 5a, with $\zeta = 0.02$ .
- **SM Movie 8**: Vortex-lattice selection in the presence of extensile active stresses and renewal: Heatmap of the polar field $p$. Scale bar: unit length. Same parameters as Fig. 5b, with $\zeta = 5 \cdot 10^{-4}$.
- **SM Movie 9**: Aster-lattice selection in the presence of contractile active stresses and renewal: Heatmap of the polar field $p$. Scale bar: unit length. Same parameters as Fig. 5b, with $\zeta = -5 \cdot 10^{-4}$.

- **SM Movie 10**: Spaghetti phase in the presence of extensile active stresses and renewal: Heatmap of the polar field $p$. Scale bar: unit length. Same parameters as in Fig. 5a, except for $\zeta = 5 \cdot 10^{-3}$ and $\tau^{-1} = 5$.


[1] L. Dumoulin, C. Blanch-Mercader, and K. Kruse, arXiv preprint arXiv:2506.03795 (2025).
[2] K. Kruse, J.-F. Joanny, F. Jülicher, J. Prost, and K. Sekimoto, The European Physical Journal E **16**, 5 (2005).
[3] A. C. Callan-Jones and F. Jülicher, New Journal of Physics **13**, 093027 (2011).
[4] S. Fürthauer, M. Neef, S. W. Grill, K. Kruse, and F. Jülicher, New Journal of Physics **14**, 023001 (2012).
[5] T. Besard, C. Foket, and B. De Sutter, IEEE Transactions on Parallel and Distributed Systems 10.1109/TPDS.2018.2872064 (2018), arXiv:1712.03112 [cs.PL].
[6] T. Besard, V. Churavy, A. Edelman, and B. De Sutter, Advances in Engineering Software **132**, 29 (2019).
[7] F. Vafa and A. Doostmohammadi, Europhysics Letters (2025).
